# Supplementary material for: Rethinking Learning-based Demosaicing, Denoising, and Super-Resolution Pipeline
Source: arXiv:1905.02538 source file (2023-03-24)
Supplement: Supplementary file 1 [file supplementary.tex]

\setcounter{section}{0}

In this supplementary material, We conclude the main paper with these additional materials:
\begin{itemize}
    \item Ablation study on the noise model; 
    \item Ablation study on the SR factor; 
    \item Exemplary images of our PixelShift200 dataset;
    \item Future work.
\end{itemize}

\subsection{Examples Images from PixelShift200}
We show the all the testing images (20 images in total) of PixelShift200 Test in \figurename~\ref{fig:supp:pixelshift200test}. We will also opensource the PixelShift200 dataset in our website. 

\begin{figure*}
\includegraphics[width=\textwidth]{imgs-s/pixelshift200/pixelshift200test.jpg}
\caption{The preview of the 20 images on PixelShift200 Test set. }
\label{fig:supp:pixelshift200test}
\end{figure*}

\subsection{Future Work}
In this paper, we focus on the pipeline of the mixture problem of DN, DM and SR. We discovered that simply changing the execution order has a significant impact on the image quality regardless of the architecture, the dataset, the noise model and the SR factor. Our findings indicate that raw image super-resolution is a promising research area that is currently under-explored. For example, a better architecture specially designed for raw image SR is deserving more research attention. In addiition, our proposed real-world full color sampled dataset PixelShift200 can be served as a good benchmark for demosaicing. We leave that as a future work as well.
